# Supplementary material for: Read, Look or Listen? What's Needed for Solving a Multimodal Dataset
Source: arXiv:2307.04532 source file (2023-07-06)
Supplement: Supplementary file 1 [file 2c-classifiers_flaw.tex]

\cref{tab:three_tasks_results_app_2} presents an evaluation of the classifiers' performance on misclassified and classified data from the original Merlot model on the TVQA dataset. The analysis reveals a decline in performance across almost all modalities when assessing the misclassified questions. This decline can be attributed to the classifiers' input being dependent on the output of the Merlot model, which is limited by its ability to accurately answer the questions. However, future developments in multi-modal models may result in more dependable classifiers.

\begin{table*}[!htb]
\caption{\label{tab:three_tasks_results_app_2} The accuracy of the classifiers on misclassified or classified questions by the Merlot model in the original TVQA is shown in the table for the validation, test, and out-of-distribution (OOD) sets of the classifiers.}
\centering
\begin{tabular}{@{}p{0.001cm}p{1.4cm}cccccccccc@{}} \toprule
\multicolumn{2}{l}{} & 
\multicolumn{3}{c}{Image} & 
\multicolumn{3}{c}{Text} & 
\multicolumn{3}{c}{Audio}  
\\ \cmidrule(l){3-5} \cmidrule(l){6-8} \cmidrule(l){9-11} 
\multicolumn{1}{l}{}     &Data  & Val & Test  & OOD   & Val  & Test  & OOD  & Val  & Test  & OOD \\ \midrule

& classified             
& \phantom{0} 91              & \phantom{0} 82                & \phantom{0} 82              & \phantom{0} 85              & \phantom{0} 79               & \phantom{0} 81               
& \phantom{0} 81              & \phantom{0} 76               & \phantom{0} 78  \\

& mis
& \phantom{0} 78              & \phantom{0} 75                & 
\phantom{0} 70              & 
\phantom{0} 73              &
\phantom{0} \textbf{54}               & 
\phantom{0} 75               &
\phantom{0} 85              & 
\phantom{0} 73               & 
\phantom{0} 70  \\

\midrule & all
& \phantom{0}\textbf{89}              & \phantom{0}81                &
\phantom{0}\textbf{80}              & 
\phantom{0} \textbf{82}              & 
\phantom{0} 74               & 
\phantom{0} \textbf{80}               & 
\phantom{0} \textbf{81}              &
\phantom{0} 76               & \phantom{0}77  \\
\end{tabular}

\end{table*}
